# Supplementary material for: Cheesecloth: Zero-Knowledge Proofs of Real-World Vulnerabilities
Source: arXiv:2301.01321 source file (2023-01-03)
Supplement: Supplementary file 1 [file appendix.tex]

\appendix

\subsection{A comprehensive discussion of system calls}
\label{app:more-system-calls}

\SC{discuss syscalls in detail}
